# Supplementary material for: Projection onto quadratic hypersurfaces
Source: arXiv:2204.02087 source file (2022-04-05)
Supplement: Supplementary file 1 [file appendix.tex]

\appendix

\section{Formulation of the projection onto the quadric as a standard form}%
\label{sec:Formulation_of_the_projection_onto_the_quadric_as_a_standard_form}

	We define the quadric manifold. Then, we use it to define the extended quadric manifold.

	\begin{proposition}[Quadric manifold]
		\label{prop:quadric_manifold}
		Let $\Psi : \mathbb{R}^n \to \mathbb{R}: \pt \mapsto \Psi(\pt) = \Tr{\pt} \B \pt + \Tr{\Ab} \pt + \Ac_t$, be a quadratic function. If $\A$ is nonsingular and $\Ac_t \neq \Tr{\Ab} \B^{-1} \Ab$, then the quadric $\mathcal{Q}(\Psi)$ is an $n-1$ dimensional smooth manifold of $\mathbb{R}^n$.
\end{proposition}

Let us start from the initial quadric equation, 
\begin{equation}
	\Tr{\x} \A \Tr{\x} + \Tr{\Ab} \x + \Ac = 0
\end{equation}

\begin{enumerate}
	\item[\textbf{Shift}] We shift the quadric such that its middle point $\d = - \frac{-\A^{-1} \Ab}{2} $ is $\bm 0$. Let $\y = \x - \d$ we have

		\begin{align*}
			0 &= \Tr{\x} \A \Tr{\x} + \Tr{\Ab} \x + \Ac \\
			0 &= \Tr{(\y + \d)} \A \Tr{(\y + \d)} + \Tr{\Ab} (\y + \d) + \Ac \\
			0 &= \Tr{\y} \A \Tr{\y} +\underbrace{ \Tr{\d} \A \d + \Tr{\Ab} \d + \Ac}_{:= \gamma} \\
		\end{align*}
		Alternatively, this is equivalent to removing the linear term.
	\item[\textbf{Scaling}] We scale the quadric, to obtain the standard form:
		\begin{equation}
			1 = \Tr{\z} \A \z 
		\end{equation}
		with $\z = \frac{y}{\sqrt{\abs{\gamma}}} $ and assuming $\gamma < 0$ which is the case in the economic dispatch.

	\item[\textbf{Rotating}] Finally, we rotate the axes to align it with the principal directions if $\A = \bm V \bm \Lambda \Tr{\bm V}$ is the diagonalization of $\A$, then we have
		\begin{align*}
			1 &= \Tr{\Tr{\bm V} \z} \bm \Lambda  \Tr{\bm V} \z \\
			1 &= \Tr{\bm u} \bm \Lambda \bm u \\
			1 &= \sum_{i = 1}^n u_i^2 \lambda_i \\
			1 &= \sum_{i = 1}^n \left(\frac{u_i}{\frac{1}{\sqrt{\lambda_i}}}\right)^2  \textrm{sign}(\lambda_i) \\
		\end{align*}
		For the ellipse, a parametrization is simply
		\begin{equation}
			(x_1(t), x_2(t)) = (\frac{1}{\sqrt{\lambda_1}}\cos t, \frac{1}{\sqrt{\lambda_2}}\sin t)
		\end{equation}
		For the hyperbola, and $\lambda_1 > 0 > \lambda_2$, a parametrization is simply
		\begin{equation}
			(x_1(t), x_2(t)) = (\frac{1}{\sqrt{\lambda_1}}\sec t, \frac{1}{\sqrt{\lambda_2}}\tan t)
		\end{equation}

\end{enumerate}

\section{Exact projection onto quadric in normal form}%
\label{sec:Exact_projection_on_quadric}

\subsection{Quadric is a sphere}%
\label{sub:Quadric_is_a_sphere}

Let us assume the quadric is a sphere, \ie, we are interested in the following problem

\begin{align*} \label{eq:proj_sphere}
	\min_{\bm x \in \Rn} 	& \norm{\bm x - \bm x^0}_2^2 \\ \numberthis
	\text{s.t. } 	& \Tr{\x} \x + \Tr{\Ab}\x + c =0 , \\
\end{align*}
and the quadric matrix $\A = \bm I$.

\begin{proposition}[Optimality of the quasi-projection onto the sphere] \label{prop:optimality_sphere_0}
	If $\A = \bm{I} \text{ and }\x^0 \neq -\frac{b}{2}$, then the two points $\x^0 + \beta^+ \bm \xi$ and $\x^0 + \beta^- \bm \xi$ from~\cref{alg:quasi-projection-quadric} are the minimum and maximum of~\cref{eq:proj_quadric}.
\end{proposition}

Similarly, the quasi-projection is optimal in the ellipsoid case, if we use the non canonical norm induced by the matrix $\A$. Indeed if $\A \succ \bm{0}$ then the mapping
\[
	\left | \left | \cdot \right | \right |_{\A} = \Rn \to \mathbb{R} : \bm{x} \mapsto  \norm{\bm{x}}_{\A} := \sqrt{\Tr{\bm x} \A \bm{x}}
\]
is a \emph{vector norm} on $\Rn$. Note that such a formulation has applications in, \eg, the training of support vector machines (SVM) using the Mahalanobis distance~\cite{tsang_2006}, and graph bisections~\cite{wang_fast_2013}.

\begin{proposition}[Optimality of the quasi-projection onto the ellipsoid] \label{prop:optimality_ellipsoid_0}
	If $\A \succ \bm 0$ and $\x^0 \neq -\A^{-1}\frac{b}{2}$, then the two points $\x^0 + \beta^+ \bm \xi$ and $\x^0 + \beta^- \bm \xi$ from~\cref{alg:quasi-projection-quadric} are the minimum and maximum of
\begin{align*} \label{eq:proj_not_sphere_0}
	\min_{\bm x \in \Rn} 	& \norm{\bm x - \bm x^0}_{\A}^2 \\ \numberthis
	\text{s.t. } 	& \Tr{\x} \A \x + \Tr{\Ab}\x + c =0 . \\
\end{align*}
\end{proposition}

The proofs are given in~\cref{sub:Quadric_is_a_sphere,sub:Quadric_is_not_a_sphere}.

The Lagrangian function reads
\begin{equation}
	\label{eq:lagrangian_sphere}
	\mathcal{L}(\x, \mu) = \Tr{(\x - \x^0)} (\x - \x^0) + \mu(\Tr{\x} \x + \Tr{\Ab}\x +c),
\end{equation}
and the extreme points should satisfy
\begin{align*}
	\label{eq:grad_lagrangian_sphere}
	\bm \nabla \mathcal{L} (\x, \mu) 	&= \bm 0 \\
						&= \begin{pmatrix}
							2 (\x - \x^0) + 2 \mu \x + \mu \Ab \\
							 \Tr{\x} \x + \Tr{\Ab}\x + c 			
						\end{pmatrix}
\end{align*}
Isolating $\x$ in the first expression yields, for $\mu \neq -1$ and $\tilde{\Ab}:=\frac{\Ab}{2}$,

\begin{equation}
	\label{eq:aligned_grad}
	\x = \frac{- \mu \Ab + 2 \x^0 }{2(1+\mu)} =  \frac{-\mu \tilde{\Ab} + \x^0 }{(1+\mu)} ,
\end{equation}
inserting it in the second expression, we obtain a second order quadratic equation in terms of $\mu$, \ie,
\begin{align*}
	\Tr{\left (\frac{-\mu \tilde{\Ab} + \x^0 }{(1+\mu)}\right)} \left ( \frac{-\mu \tilde{\Ab} + \x^0 }{(1+\mu)} \right ) + \Tr{\Ab}  \left ( \frac{-\mu \tilde{\Ab} + \x^0 }{(1+\mu)} \right ) + c &= 0	\\
\Tr{\left (-\mu \tilde{\Ab} + \x^0 \right)} \left (- \mu \tilde{\Ab} + \x^0 \right ) + \Tr{\Ab}  \left ( -\mu \tilde{\Ab} + \x^0 \right ) (1+\mu) + c (1+\mu)^2 &= 0	\\
\mu^2 \Tr{\tilde{\Ab}} \tilde{\Ab} - 2\mu \Tr{\tilde{\Ab}} \x^0 + \Tr{\x^0}\x^0 - \mu \Tr{\Ab} \tilde{\Ab} + \Tr{\Ab} \x^0 - \mu^2 \Tr{\Ab} \tilde{\Ab} + \mu \Tr{\Ab} \x^0 +c \mu^2 + 2c\mu + c &=0 \\
\mu^2 (\Tr{\tilde{\Ab}} \tilde{\Ab} - \Tr{\Ab}\tilde{\Ab}+c ) + \mu (-2\Tr{\tilde{\Ab}}\x^0- \Tr{\Ab}\tilde{\Ab}+\Tr{\Ab} \x^0+2c) + \Tr{\x^0}\x^0 + \Tr{\Ab}\x^0 + c &= 0 \\
\mu^2 \underbrace{( - \frac{\Tr{\Ab}\Ab}{4}+c )}_{:=a_1} + \mu \underbrace{(- \Tr{\Ab}\tilde{\Ab}+2c)}_{:=a_2} + \underbrace{\Tr{\x^0}\x^0 + \Tr{\Ab}\x^0 + c}_{:=a_3} &= 0 \\
\end{align*}

and providing that $a_1 \neq 0$, the two solutions $\mu^+, \, \mu^-$ are
\begin{equation}
	\label{eq:lambda_sphere_case}
	\mu = \frac{-a_2 \pm \sqrt{a_2^2 - 4 a_1 a_3}}{2 a_1}.
\end{equation}
Note that if $\mu =-1$, then the first equation from the gradient of the Lagrangian yields $\x^0 = -\frac{b}{2} $. This situation correspond to the case when the initial point $\x^0$ \emph{is the middle point of the sphere}. In this situation, \emph{any feasible point is the optimal solution}.

Let us now show that the solution of the geometric construction from~\cref{alg:quasi-projection-quadric} is the exact projection, \ie, the point $\x(\mu)$ from~\cref{eq:aligned_grad} with the optimal $\mu$ given by~\cref{eq:lambda_sphere_case}.

We begin with a Lemma linking the optimal Lagrange parameter $\mu$ given by~\cref{eq:lambda_sphere_case} with the optimal shift $\beta$ from~\cref{alg:quasi-projection-quadric}. 

\begin{lemma}
	\label{lemma:lambda_beta_sphere}
	Given parameters $\mu :=\mu^+$ and $\beta :=\beta^-$ from~\cref{alg:quasi-projection-quadric} and~\cref{eq:lambda_sphere_case}, if $x^0 \neq -\frac{\Ab}{2}$ and $b_2^2 - 4 b_1 b_3 > 0$ then 
$$\mu + \beta + \mu \beta = 0 . $$
\end{lemma}
\begin{proof}
	The first assumption on $x^0$ lets us avoid the degenerate case when the point to be projected is the middle point of the sphere, such case has been discussed in \S~\ref{sub:Quadric_is_a_sphere}. The second assumption is a technical assumption \textcolor{red}{To be discussed}

	First, if we consider the $a_i$'s and $b_i$'s from both methods, we note that since $\A = \bm I$,
	\begin{align*}
		a_1 &= \frac{a_2}{2} := a, \\
		b_1 &= \frac{b_2}{2} := b, \\
		a_3 &= b_3 := \delta, \\
		\delta &= a + b.
	\end{align*}
	Remark that since $b = \norm{\bm \xi}_2^2$, we have $b> 0$ and therefore, using the technical assumption, we have $a < 0$.
	Hence, we compute
	\begin{align*}
		\mu &= -1 - \sqrt{-\frac{b}{a}} \quad \text{since } a < 0, \\
		\beta	&= -1 - \sqrt{-\frac{a}{b}} \quad \text{since } b > 0,\\
	\end{align*}
	and it follows that
	\begin{align*}
		\mu + \beta 	&= -2 - \sqrt{-\frac{b}{a}} - \sqrt{-\frac{a}{b}}, \\
		\mu \beta 		&= 1 + \sqrt{-\frac{b}{a}} + \sqrt{-\frac{a}{b}} + 1.
	\end{align*}
\end{proof}

Remark that~\cref{lemma:lambda_beta_sphere} is also valid for the couple $(\mu^-, \beta^+)$, and the proof is similar.

Using~\cref{lemma:lambda_beta_sphere}, we can prove that the geometric construction is optimal if the quadric is a sphere.

\begin{proposition}[Optimality of the quasi-projection onto the sphere] \label{prop:optimality_sphere}
	If $\x^0 \neq -\frac{b}{2}$, then the two points returned by~\cref{alg:quasi-projection-quadric} are the minimum and maximum of~\cref{eq:proj_sphere}.
\end{proposition}
\begin{proof}
	Let us first assume that the technical assumption $a_2^2 - 4 a_1 a_3 > 0$ is verified. \textcolor{red}{To proof or add as assumption}
	Using~\cref{lemma:lambda_beta_sphere}, we have successively
	\begin{align*}
		\mu + \beta + \mu \beta &= 0 \\
		(\mu + \beta) (\x^0+\frac{\Ab}{2}) + \mu \beta(\x^0+ \frac{\Ab}{2}) &= 0 \\
		\x^0 (\mu + \beta) + \mu \beta (\x^0 + \frac{\Ab}{2}) + \frac{\Ab}{2} (\mu + \beta) &= 0 \\
		\x^0 + \mu \x^0 + \beta \x^0 + \beta \frac{\Ab}{2} + \mu \beta \x^0 + \mu \beta \frac{\Ab}{2} &= \x^0 - \mu \frac{\Ab}{2}\\
		\x^0 + \beta (\x^0 + \frac{\Ab}{2}) &= \frac{\x^0 - \mu \frac{\Ab}{2}}{1+\mu} \\
		\x^0 + \beta (\x^0 - \d) &=\frac{\x^0 - \mu \frac{\Ab}{2}}{1+\mu} \\
		\x^0 + \beta \bm \x^0 &= \frac{\x^0 - \mu \frac{\Ab}{2}}{1+\mu} \\
	\end{align*}
	Hence the points returned by~\cref{alg:quasi-projection-quadric} \emph{are zeros of the Lagrangian function} of~\cref{eq:proj_sphere}. \textcolor{red}{add argument that it is the min and the max... Via slater ? I don't think so because the problem is not convex}. Moreover, as the feasible set of problem~\cref{eq:proj_sphere} is compact, by the Weierstrass extreme value theorem, the objective~\cref{eq:proj_sphere} obtains its extreme values. These extreme values should belong either to the set of the zeros of the Lagrangian, or to the zero-set of the constraint gradient. Since we have exactly two zeros of the Lagrangian, and because the only root of the constraint gradient is $-\frac{\Ab}{2}$, which does not belong to the sphere by assumption, we can conclude that the two roots are the minimum and maximum value of problem~\cref{eq:proj_sphere}.
\end{proof}

\subsection{Quadric is not a sphere}%
\label{sub:Quadric_is_not_a_sphere}

\textcolor{red}{Could I simply use the change of variable $\bm y = \bm L \bm x$ where $\bm L$ is the Cholesky decomposition of $\A$ and conclude that it is simiar as~\cref{sub:Quadric_is_a_sphere}? }

Let us assume the quadric is \emph{not} a sphere, \ie, we are interested in the following problem

\begin{align*} \label{eq:proj_not_sphere}
	\min_{\bm x \in \Rn} 	& \norm{\bm x - \bm x^0}_{\A}^2 \\ \numberthis
	\text{s.t. } 	& \Tr{\x} \A \x + \Tr{\Ab}\x + c =0 . \\
\end{align*}

The Lagrangian function reads
\begin{equation}
	\label{eq:lagrangian_not_sphere_quasi}
	\mathcal{L}(\x, \mu) = \Tr{(\x - \x^0)} \A (\x - \x^0) + \mu(\Tr{\x} \A \x + \Tr{\Ab}\x +c),
\end{equation}
and the extreme points should satisfy
\begin{align*}
	\label{eq:grad_lagrangian_not_sphere_quasi}
	\bm \nabla \mathcal{L} (\x, \mu) 	&= \bm 0 \\
						&= \begin{pmatrix}
							2 \A(\x - \x^0) + 2 \mu \A \x + \mu \Ab \\
							 \Tr{\x} \A \x + \Tr{\Ab}\x + c 			
						\end{pmatrix}
\end{align*}
Isolating $\x$ in the first expression yields, for $\mu \neq -1$ and $\tilde{\Ab}:=\frac{\Ab}{2}$,

\begin{equation*}
	\label{eq:aligned_grad_not_sphere}
	\x =\A^{-1}  \frac{2 \A \x^0 - \mu \Ab }{2(1+\mu)} =   \frac{ \x^0 - \mu \A^{-1}\tilde{\Ab} }{(1+\mu)} ,
\end{equation*}

Working in a similar way as the sphere case, we obtain the two extrema. Note that the same comment also holds for $\mu = -1$: a problem occur if $\x^0 = - \frac{\A^{-1}\Ab}{2}$, \ie, if the initial point is the quadric middle point. In this case, any point of the ellipsoid is also an optimal solution. Indeed given the norm $\norm{\cdot}_{\A}$, our ellipsoid is the corresponding ball.

The optimal $\mu$ satisfy the following equality

\begin{equation*}
	\mu^2 \underbrace{( - \frac{\Tr{\Ab} \A^{-1} \Ab}{4}+c )}_{:=a_1} + \mu \underbrace{(- \Tr{\Ab} \A^{-1} \tilde{\Ab}+2c)}_{:=a_2} + \underbrace{\Tr{\x^0} \A \x^0 + \Tr{\Ab}\x^0 + c}_{:=a_3} = 0, 
\end{equation*}
 and the two solutions $\mu^+, \, \mu^-$ are

\begin{equation}
	\label{eq:lambda_ellipsoid_case}
	\mu^{+,-} = \frac{-a_2 \pm \sqrt{a_2^2 - 4 a_1 a_3}}{2 a_1}.
\end{equation}

Similarly to the sphere case, we can prove that the geometric construction of~\cref{alg:quasi-projection-quadric} yields the two optimum of~\cref{eq:proj_not_sphere}.

\begin{lemma}
	\label{lemma:lambda_beta_ellipse}
	Given parameters $\mu :=\mu^+$ and $\beta :=\beta^-$ from~\cref{alg:quasi-projection-quadric} and~\cref{eq:lambda_ellipsoid_case}, if $x^0 \neq -\frac{b}{2}$ and $b_2^2 - 4 b_1 b_3 > 0$ then 
$$\mu + \beta + \mu \beta = 0 . $$
\end{lemma}
\begin{proof}
	If we consider the $a_i$'s and $b_i$'s from both methods, we note that since $\d = -\A^{-1} \frac{\Ab}{2} $,
	\begin{align*}
		a_1 &= \frac{a_2}{2} := a, \\
		b_1 &= \frac{b_2}{2} := b, \\
		a_3 &= b_3 := \delta, \\
		\delta &= a + b.
	\end{align*}
	and since the $\mu$'s and $\beta$'s have the same dependence with respect to the $a_i$'s and $b_i$'s as in~\cref{lemma:lambda_beta_sphere}, the proof is identical.

\end{proof}

Since the Lemma is valid in the ellipsoid case, we can use the same argument as in the proof of~\cref{prop:optimality_sphere} and conclude that

\begin{proposition}[Optimality of the quasi-projection onto the ellipsoid]
	If $\x^0 \neq -\A^{-1}\frac{b}{2}$, then the two points returned by~\cref{alg:quasi-projection-quadric} are the minimum and maximum of~\cref{eq:proj_not_sphere}.
\end{proposition}

\paragraph{Remark}%
\label{par:Remark}
Such construction works only if the bilinear form \[ \langle \cdot , \cdot \rangle: E \times E \to \mathbb{R}  : (\bm u, \bm v) \mapsto \langle \bm u, \bm v \rangle :=\Tr{\bm u} \A \bm v \]
is an inner product. This is true on $E = \Rn$ iff $\A \succ 0$, the main problem comes from the positive definiteness property, \ie, we want our bilinear form to satisfy the following property \[ \langle \bm u, \bm u \rangle > 0  \text{ if } \bm u \neq 0 .\]

However this can be true if we restrict $E$ to some linear subspace of $\Rn$.

For instance, assume $\A = \begin{pmatrix}
	1 & 0 \\
	0 & -2
\end{pmatrix}$ then the positive definiteness property holds for $E = \left \{ (x,y) \in \mathbb{R}^2 \st{x\geq \sqrt{2} y} \right \}$, note that we should make sure that it stays a linear (sub-)space... which is not the case ... It is a cone (try multiplying with a negative scalar)

\begin{figure}
	\begin{subfigure}[t]{.5\textwidth}
		\centering
		\includegraphics[width=.9\columnwidth]{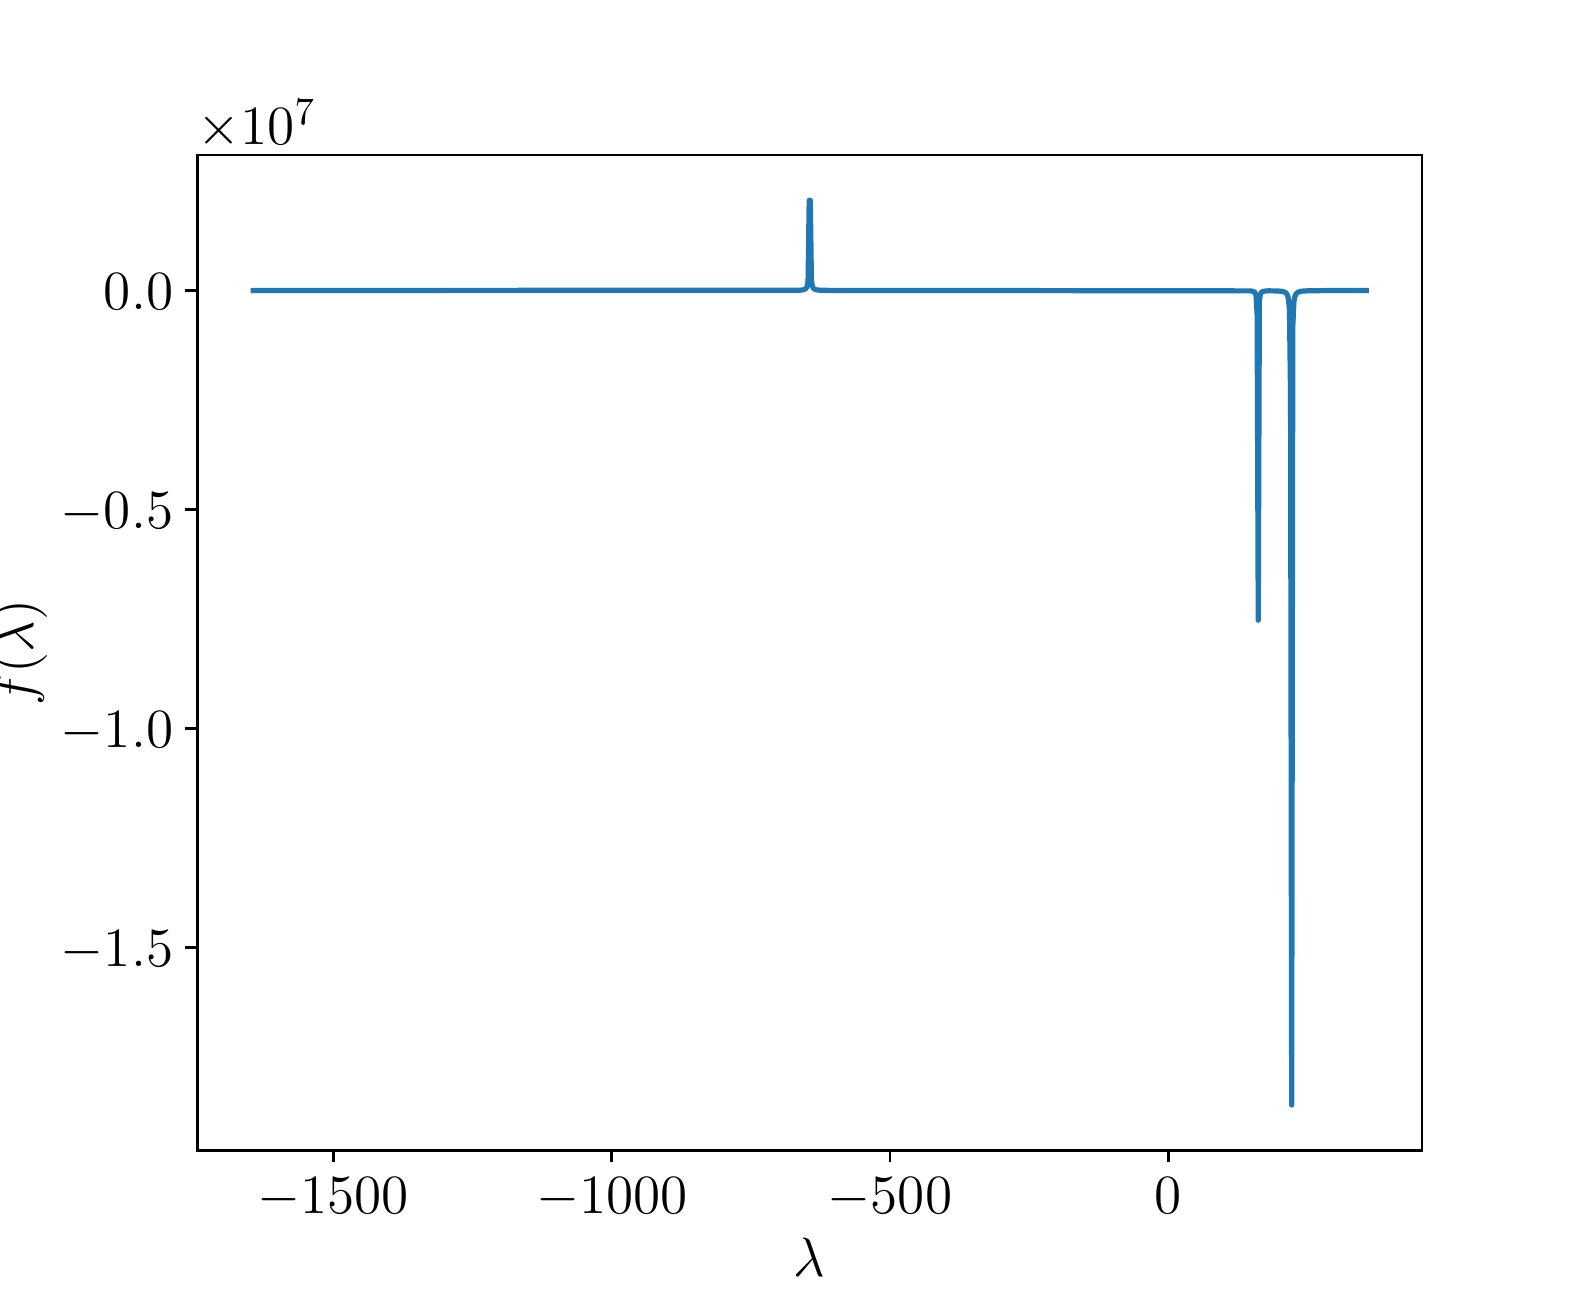}
		\caption{Full plot around the maximum.}
		\label{fig:lambda_full}
	\end{subfigure}%
	\hfill
	\begin{subfigure}[t]{.5\textwidth}
		\centering
		\includegraphics[width=.9\columnwidth]{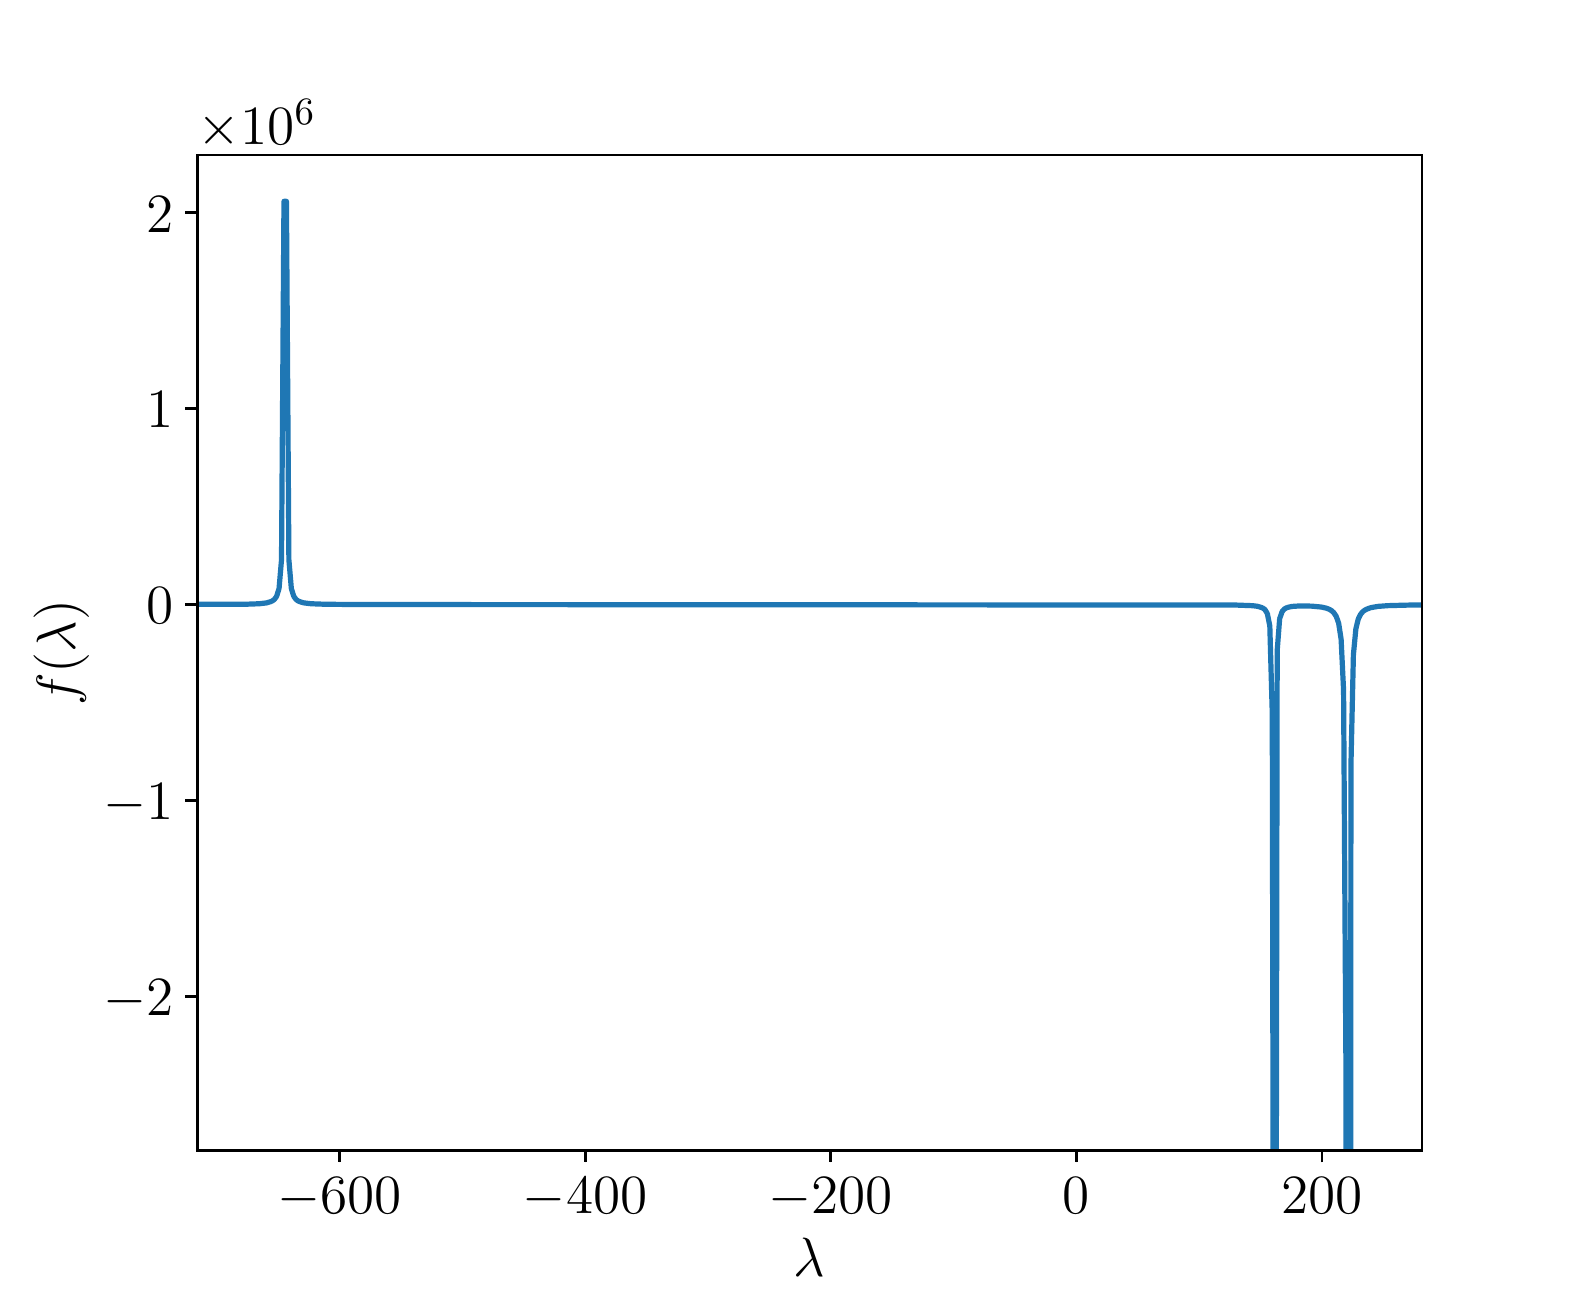}
		\caption{Magnification to observe the 3 peaks.}
		\label{fig:lambda_full_zoomed}
	\end{subfigure}
	\caption{Plot of~\cref{eq:objective_lambda} for a 3-dimension problem.}
	\label{fig:lambda}
\end{figure}

\subsection{Exact projection}%
\label{sub:Exact_projection}

Using a similar argument as the proofs from~\cref{sub:Quadric_is_a_sphere,sub:Quadric_is_not_a_sphere}, we can characterize the exact solutions~\cref{eq:proj_quadric}.

It this case the Lagrangian of~\cref{eq:proj_quadric} reads

\begin{equation}
	\label{eq:lagrangian_not_sphere_v2}
	\mathcal{L}(\x, \mu) = \Tr{(\x - \x^0)} (\x - \x^0) + \mu(\Tr{\x} \A \x + \Tr{\Ab}\x +c),
\end{equation}
and the gradient,
\begin{align*}
	\label{eq:grad_lagrangian_not_sphere_v2}
	\bm \nabla \mathcal{L} (\x, \mu) 	&= \bm 0 \numberthis\\
						&= \begin{pmatrix}
							2 (\x - \x^0) + 2 \mu \A \x + \mu \Ab \\
							 \Tr{\x} \A \x + \Tr{\Ab}\x + c 			
						\end{pmatrix}
\end{align*}

Isolating $\x$ in the first expression yields, for $\tilde{\Ab}:=\frac{\Ab}{2}$,

\begin{equation}
	\label{eq:x_not_sphere_apx}
	\x (\mu) =(\bm I + \mu \A)^{-1}  \frac{2\x^0 - \mu \Ab }{2} = (\bm I + \mu\A)^{-1}  (\x^0 - \mu \tilde{\Ab})  .
\end{equation}

Note that we enforce that $\mu \notin -\frac{1}{\rho( \A )}$, because in this case the matrix $(I + \mu \A)$ is not invertible. \textcolor{red}{To add: where do we discuss about the case of $\mu \in \mathcal{E}$ }

Inserting it in the quadric equation $\Psi$, we obtain a \emph{scalar}, \emph{real-valued} function
\begin{equation}
	\label{eq:f_mu_full}
	f : \mathbb{R} \to \mathbb{R} : \mu \mapsto f(\mu) = \Psi(\x(\mu)) = \Tr{\x(\mu)} \A \x(\mu) + \Tr{\Ab}\x(\mu) + \Ac 			
\end{equation}
whose we want to obtain the roots.

This can solved for $\mu$ by dichotomy. This raises the following points:
\begin{enumerate}
	\item This dichotomy procedure typically requires a lot of function evaluations, which are not cheap because of the inverse function in~\cref{eq:x_not_sphere};
	\item \cref{eq:grad_lagrangian_not_sphere_v2} may have several solutions corresponding to minima, maxima, or saddle points;
	\item Solving by dichotomy demands an interval $[a, b]$ with $a < b$ and $f(a) f(b) <0$.
\end{enumerate}

The first point is tackled by noticing that our matrix is diagonalizable $\A = \bm Q \bm \Lambda \Tr{\bm Q}$ with $\bm Q$ unitary. Therefore we have, $(\bm I + \mu \A)^{-1} = (\bm Q \bm Q^T + \mu \A)^{-1} = (\bm Q (\bm I + \mu \bm \Lambda ) \Tr{\bm Q})^{-1} = \bm Q (\bm I + \mu \bm \Lambda )^{-1} \Tr{\bm Q}$, which is much easier to evaluate given $\mu$.

Concerning the non uniqueness of the solution of~\cref{eq:grad_lagrangian_not_sphere_v2}, we remark that $\x (\mu)$ is a discontinuous function that rockets when $\mu \in \mathcal{E} := \tau(\A):= \left\{ -\frac{1}{\lambda} \st{\lambda \in \rho(\A)} \right \}$, where $\rho(\A)$ is the set of eigenvalues of $\A$. Note that this set is real valued,  because $\A$ is symmetric, and well-defined, because $\A$ is not singular and thus $0 \notin \rho(\A)$. Since $\x(\mu)$ rockets in the neighbourhood of any element of $\mathcal{E}$, so is the function $f(\mu)$. Hence, these discontinuity points are good candidates for finding a dichotomy interval. .

An exhaustive search of all the roots of $f$ may be investigated, \eg, by sorting the element of $\mathcal{E}$ in ascending order and checking each interval defined with two consecutive elements. However it raises already several questions. Can we prove that the set of extrema of $f$ is $\mathcal{E}$? Once we selected a valid interval for the dichotomy, could we be sure that it contains a single root?

The answer to both questions is certainly no. Indeed in the example of~\cref{fig:mu_three_roots_zoomed}, the two extrema located around 0.3 and 0.6 yield negative value of $f$, but the function has two roots, and a local maxima in this interval. Also, an exhaustive search will be costly: testing the function at each value $e \in \mathcal{E}$ costs $\mathcal{O}(n^4)$; if we assume that the matrix product takes time on the order of $n^3$.

However, we note that i) $f(\mu)$ changes of sign around zero, \ie, if $e^-$ is the largest negative element of $\mathcal{E}$ and $e^+$ the smallest positive element of $\mathcal{E}$, then $f(e^-)> 0$  and $f(e^+)>0$ (\textcolor{red}{to be proven?}\footnote{\textcolor{red}{It seems that all the values of $\mathcal{E}$ which are negative yield positive extrema and vice versa... This may be a point to prove it}}), and  ii) we are interested in the smallest $\mu$ in absolute value (\textcolor{red}{to be proven}). Intuitively, $\mu = 0$ yields $\x(0) = \bm{x}^0$ which is the optimal solution, provided that $\x^0$ initially belongs to the quadric. These two points are validated in~\cref{fig:mu_one_root,fig:mu_one_root_zoomed,fig:mu_three_roots,fig:mu_three_roots_zoomed}: there is a root $r \in ]e^-, e^+[$ around zero and the distance between $\x(\mu)$ and $\x^0$ is smaller then elsewhere. Hence, the solution $\x (r)$ is optimal.

This gives the following procedure:

\begin{algorithm}
	\caption{Exact projection onto a quadric}
	\label{alg:exact_projection_quadric_old}
	\begin{algorithmic}
		\REQUIRE $\A$ symmetric matrix
		\STATE $\bm{Q}, \bm{\Lambda} \gets \textrm{eig}(\A)$ 
		\COMMENT{spectral decomposition of $\A$}
		\STATE $\x (\mu) \gets \bm{Q} (\bm{I} + \mu \bm{\Lambda})^{-1} \Tr{\bm{Q}} (\x^0 - \mu \frac{\Ab}{2} )$
		\STATE $f (\mu) \gets  \Tr{\x(\mu)} \A \x(\mu) + \Tr{\Ab}\x(\mu) + \Ac$
		\STATE $\mathcal{E} \gets \left \{ -\frac{1}{\lambda} \st{\lambda \in \rho(\A)} \right \} $
		\STATE $e^- \gets \max \left \{ e \in \mathcal{E} \st{e <0} \right \} $
		\STATE $e^+ \gets \min \left \{ e \in \mathcal{E}\st{e > 0} \right \} $
		\STATE $\mu^* \gets \textrm{root}(f, e^-, e^+)$ \COMMENT{Dichotomy search}
		\RETURN $\mu^*, \x(\mu^*)$
	\end{algorithmic}
\end{algorithm}

If we apply this procedure, we seem to efficiently obtain the closest point: see~\cref{fig:comparison_quasi_exact_2D}.

\paragraph{Solving with Derivative}%
\label{par:Solving_with_Derivative}

Our function of interest is

\begin{equation}
	\label{eq:objective_lambda}
	f(\x(\mu)) :=\Tr{\x(\mu)} \A \x(\mu) + \Tr{\Ab}\x(\mu) + c 			
\end{equation}
with 
\begin{equation}
	\label{eq:objective_x}
	(\bm I + \mu\A)\x(\mu) =   (\x^0 - \mu \tilde{\Ab}) 
\end{equation}

We are interested into the derivative of $f$, which can be computed as

\begin{align*}
	\frac{d f(\x(\mu))}{d \mu} 	&= \nabla_{\x} f(\x(\mu)) \cdot \frac{d \x(\mu)}{d\mu}   \numberthis \label{eq:objective_lambda_chain_rule} \\
						&= (2 \A \x(\mu) + \Ab) \cdot \left( \frac{d (I+\mu \A)^{-1}}{d \mu} (\x^0 - \mu \tilde{\bm b}) - (I+\mu\A)^{-1} \tilde{\bm b} \right) \\
						&= (2 \A \x(\mu) + \Ab) \cdot \left( -(I+\mu \A)^{-1} \frac{d (I + \mu\A)}{d \mu}  (I+\mu \A)^{-1} (\x^0 - \mu \tilde{\bm b}) - (I+\mu\A)^{-1} \tilde{\bm b} \right)\\
						&= (2 \A \x(\mu) + \Ab) \cdot \left( -(I+\mu \A)^{-1} \A  (I+\mu \A)^{-1} (\x^0 - \mu \frac{\bm b}{2}) - (I+\mu\A)^{-1} \frac{\bm b}{2} \right)\\
\end{align*}
with $\tilde{\bm b} = \frac{\bm b}{2}$.

\begin{remark}
	It is probably not smart to work with the derivative as this function is not differentiable for $\mu \in -\frac{1}{\mu(\A)}$, and it does not help the solver.
\end{remark}

\paragraph{What if we do it properly?}%
\label{par:What_if_we_do_it_properly}

Let $\mathcal{E}$, $e^-$, $e^+$ be defined as in~\cref{alg:exact_projection_quadric}, let us restrict the root search between $e^-$ and $e^+$ such that
\begin{equation}
	\label{eq:f_bar}
	\bar{f} : ]e^-, e^+[ \to \mathbb{R} : \mu \mapsto \bar{f}(\mu) = f(\mu) \, ,
\end{equation}
this function is continuous and differentiable \textcolor{red}{To be proven but seems fair}.

We know that the extrema of $\bar{f}$ satisfy

\begin{align*}
	\bm 0 = \frac{d \bar{f}(\x (\mu))}{d \mu} 	&= \Tr{\nabla_x \bar{f}} \, \x'(\mu) \\
							&= \Tr{(2 \A \x +\Ab)} \x'(\mu) \numberthis \label{eq:d_objective_lambda}
\end{align*}
and we can express $\x'(\mu)$ by using~\cref{eq:objective_x},
\begin{align*}
	\frac{d \ref{eq:objective_x}}{d \mu} &\Leftrightarrow \A \x + (\bm I + \mu \A) \x'(\mu) = \frac{-\Ab}{2} \\
						  &\Leftrightarrow (\bm I + \mu \A) \x'(\mu) = \frac{-b}{2}  - \A \x \numberthis \label{eq:d_objective_x}
\end{align*}
Injecting~\cref{eq:d_objective_x} into~\cref{eq:d_objective_lambda} yields:

\begin{equation}
	\label{eq:quadratic_form_lambda}
	\bm 0 = \Tr{\x'(\mu)} (\bm I + \mu \A) \x'(\mu) .
\end{equation}
Since it is a quadratic form, it is true if $\x'(\mu) = 0$ or if $\x'(\mu) \in \ker (\bm I+\mu \A)$.

\begin{remark}
	If $\mu=0$ then $ \frac{d \bar{f}(\x (0))}{d \mu}= \Tr{\x'(0)} \x'(0) \geq 0$: the function is increasing in $\mu=0$ and $\x(0) = \x^0$. 
\end{remark}

\begin{remark}
	What happen if I choose $\mu$ such that $\nabla_{\x} \bar{f}(\x(\mu)) = \bm 0$? It is not an issue because then it is equivalent to say that
	\[ 
		\x(\mu) = \frac{-\A^{-1} \Ab }{2} 
	\]
	and therefore injecting it into~\cref{eq:objective_x} yields
	\begin{align*}		
		-(\bm I + \mu \A) \frac{\A^{-1} \Ab}{2} &= \x^0 - \frac{\mu \Ab}{2}\\  
		- \frac{\A^{-1}\Ab}{2} - \frac{\mu \Ab}{2} &= \x^0 - \frac{\mu \Ab}{2} \\
		- \frac{\A^{-1}\Ab}{2} &= \x^0
	\end{align*}
	This last equation is also equivalent to the specific case when the initial point is the middle point of the quadric.

	Hence~\cref{eq:objective_lambda_chain_rule} is true if
	\begin{enumerate}
		\item $\x'(\mu)=\bm 0$
		\item $\x' (\mu) \perp \nabla_{\x} \bar{f} (\mu)$ 
	\end{enumerate}
\end{remark}

\begin{figure}
	\centering
	\begin{subfigure}[b]{.475\textwidth}
		\centering
		\includegraphics[width=\linewidth]{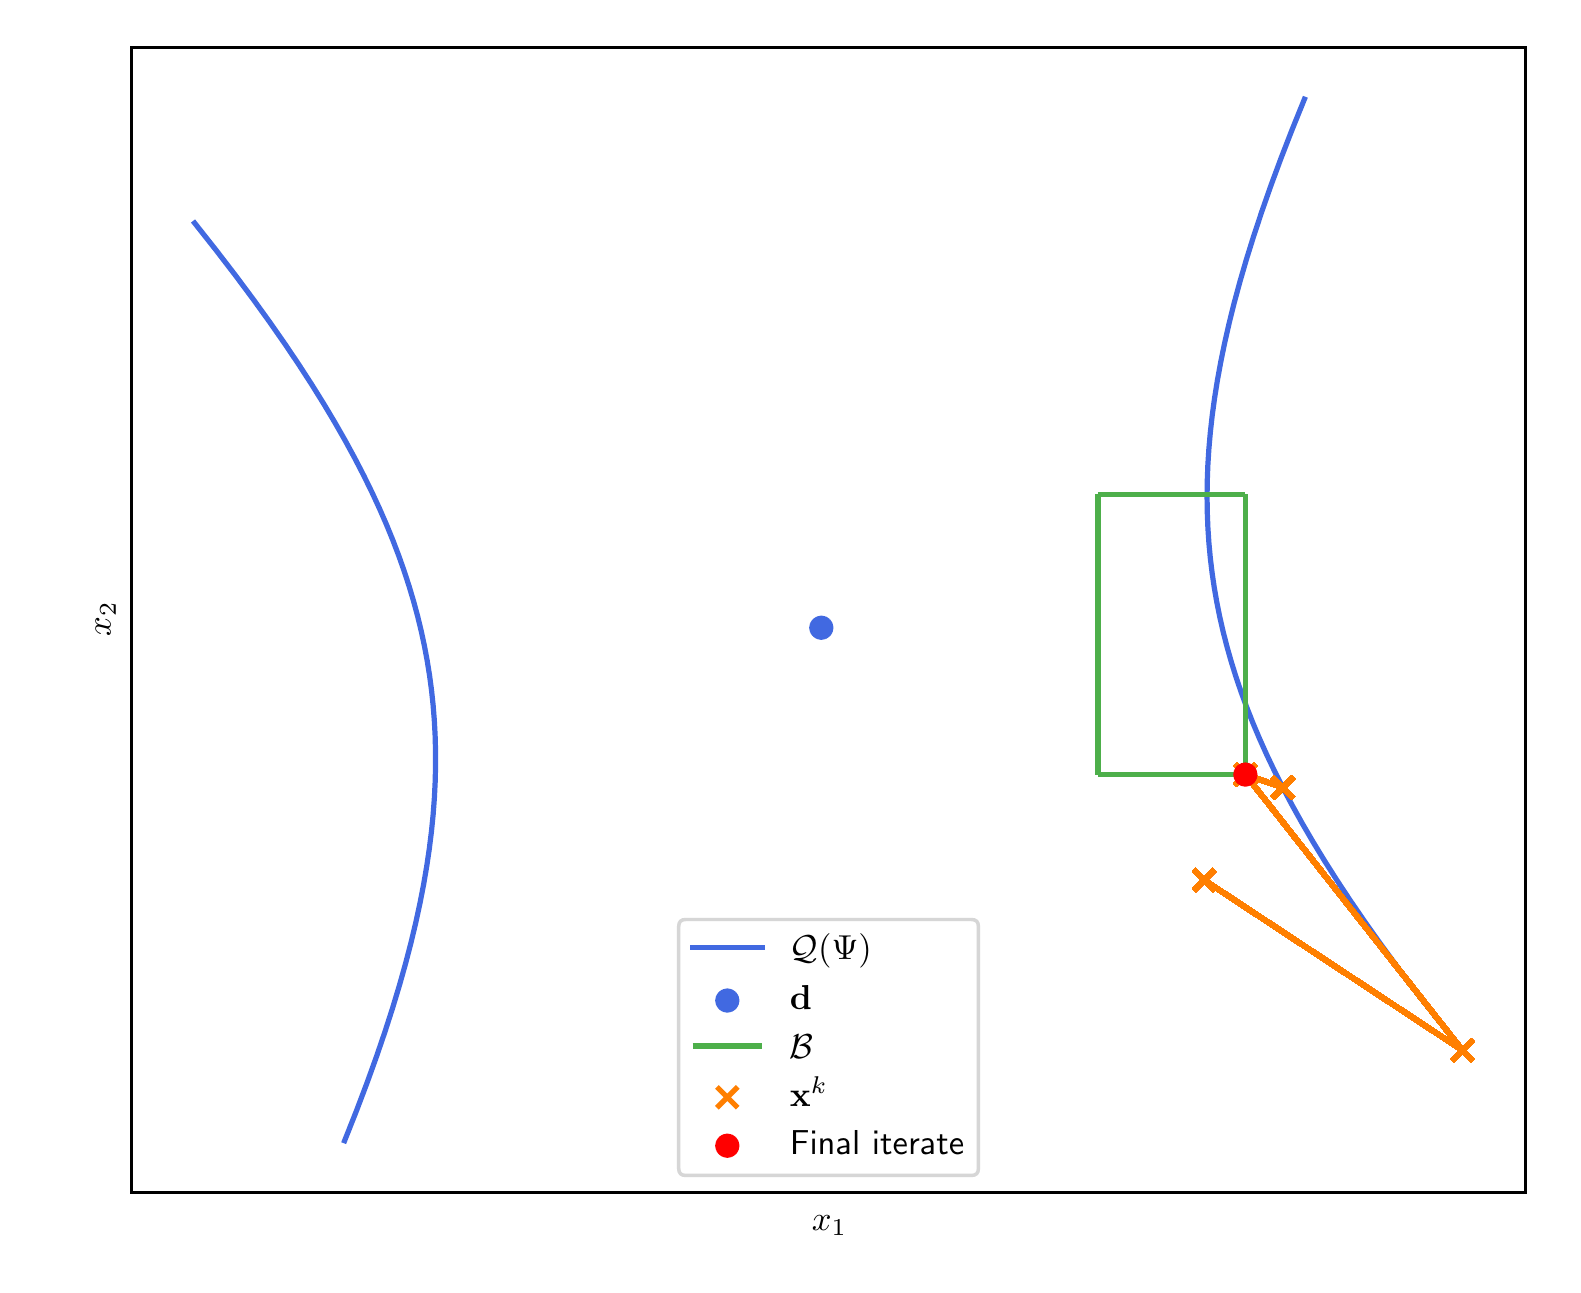}
		\caption{The method fails as it oscillates between two points.}
		\label{subfig:hyperbole_KO_corner}
	\end{subfigure}%
	\hfill
	\begin{subfigure}[b]{.475\textwidth}
		\centering
		\includegraphics[width=\linewidth]{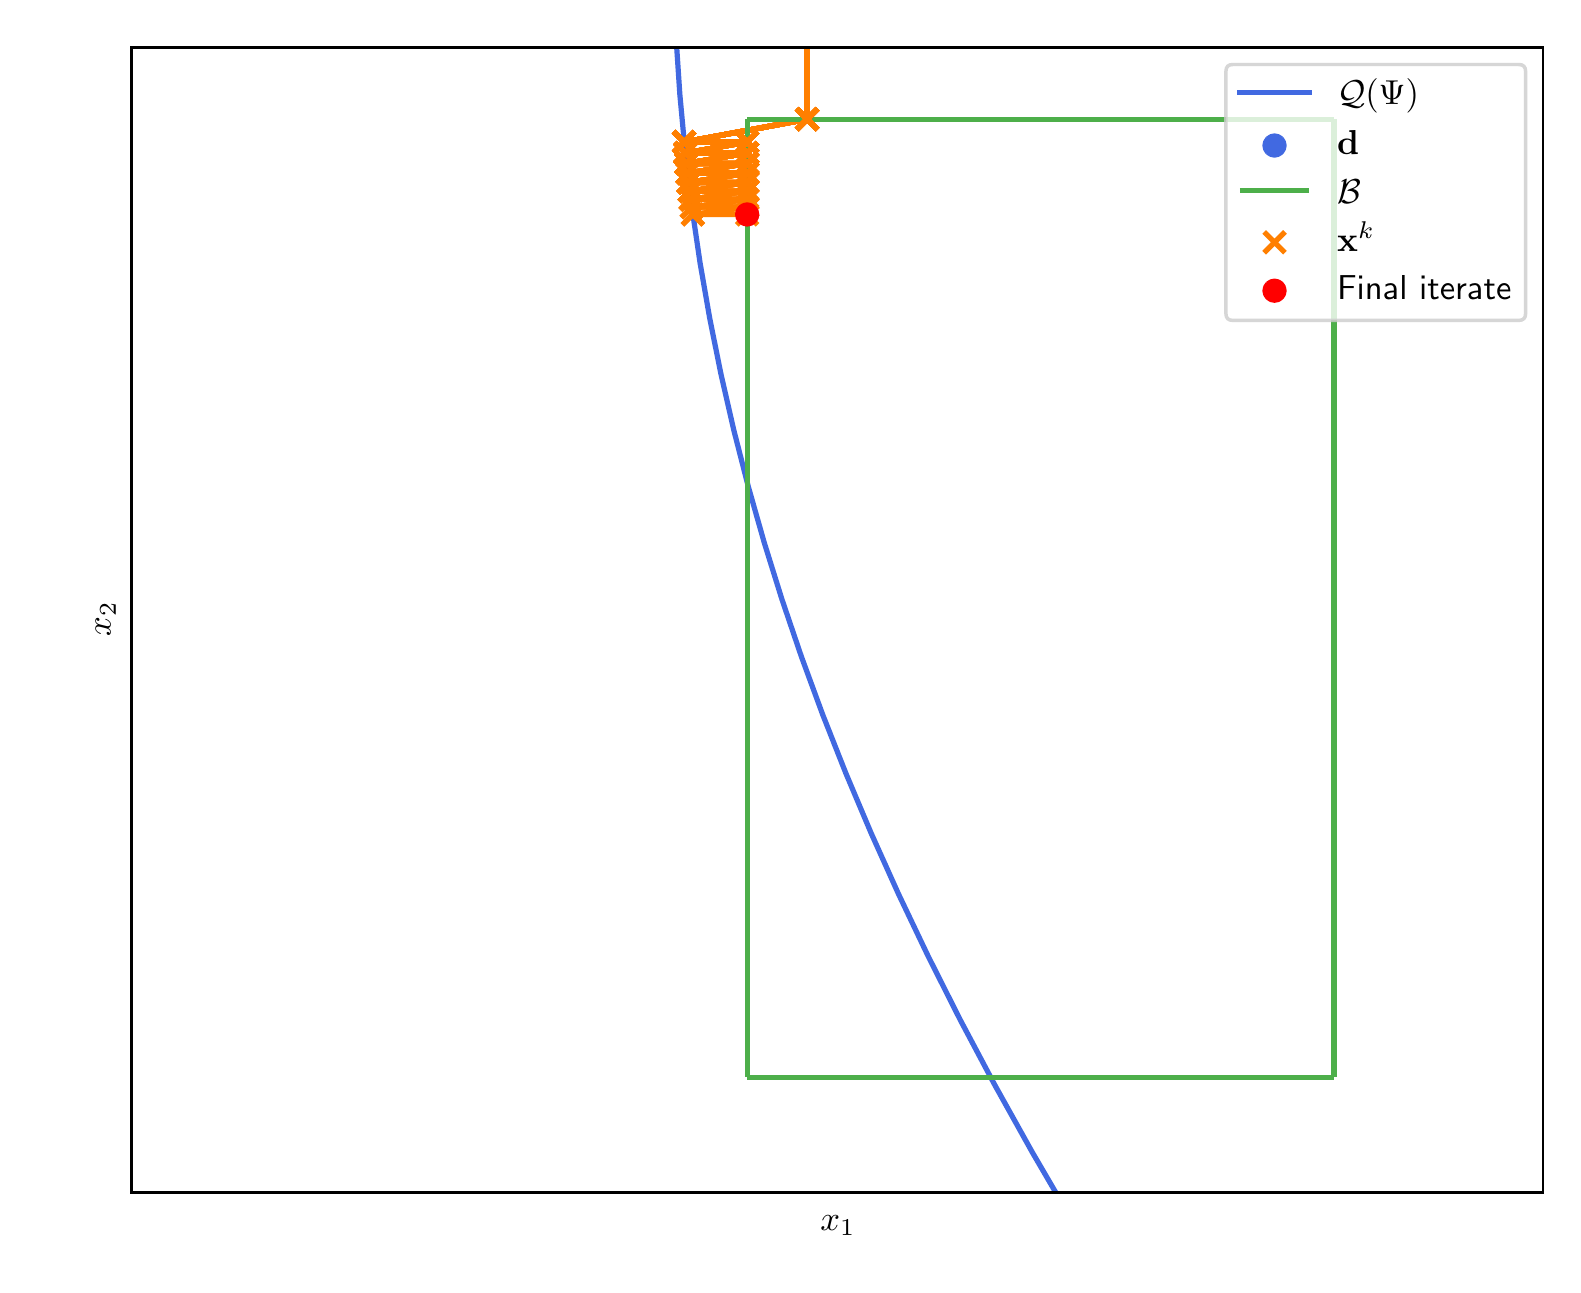}
		\caption{The method fails as it reaches the iteration limit (20 here).}
		\label{subfig:hyperbole_KO_oscillating}
	\end{subfigure}
\caption{Illustration of instances when the alternating projection method fails to return a feasible solution given an iteration limit.}
\label{fig:APC_fail}
\end{figure}
\subsection{Damped alternating projection method}%
\label{sub:Alternate_projection_method_APD}

We slightly modify~\cref{alg:quasi-projection-quadric} such that the direction used to map the point to the quadric, $\bm \xi$, can be chosen arbitrarily:

\begin{algorithm}
	\caption{Quasi-projection onto the quadric with arbitrary direction}
	\label{alg:projection-quadric-arbitrary}
	\begin{algorithmic}
		\REQUIRE{$\x^0 \in \Rn$, $\bm \xi \in \Rn$, and a type-II quadric $\Q$}
		\STATE{$b_1 \gets \Tr{\bm \xi}  \A \bm \xi$}
		\STATE{$b_2 \gets 2 \Tr{\x^0}  \A \bm \xi + \Tr{\Ab} \bm \xi $}
		\STATE{$b_3 \gets \Tr{\x^0}  \A \x^0 + \Tr{\Ab} \x^0 + \Ac$}
		\STATE{$\Delta \gets \sqrt{b_2^2 - 4 b_1 b_3}$}
		\STATE $\beta^+ \gets  \frac{-b_2 + \Delta}{2 b_1} $
		\STATE $\beta^- \gets  \frac{-b_2 - \Delta}{2 b_1} $
	\STATE $\beta \gets \argmin{ \left\{ \abs{\beta^+}, \abs{\beta^-} \right \}}$
	\COMMENT{we select the closest of the 2 intersections}
		\RETURN $\x^0 + \beta \bm \xi$
	\end{algorithmic}
\end{algorithm}

As direction $\bm \xi$, we take the gradient of the constraint~\cref{eq:quadric} of the previous iterate. This gives~\cref{alg:projection-quadric-arbitrary}.

\begin{algorithm}[h!]
	\caption{Alternating projection method}
	\label{alg:Alternate_projection_method}
	\begin{algorithmic}
		\REQUIRE $\bm x^0 \in \Rn$
		\STATE $k \gets 0$
		\STATE $\bm \xi^{0} \gets \x^0 - \d$
		\COMMENT{The first iterate is equivalent to~\cref{alg:quasi-projection-quadric}.}
		\WHILE{$k < \niter$ \textrm{\textbf{and not}} $\bm x^k \in \Omega$}
			\STATE $\bm y^{k+1} \gets \Pr_{\mathcal{B}}(\x^k)$
			\COMMENT{Using~\cref{alg:projection-box}}
			\STATE $\x^{k+1} \gets \Pr_{\mathcal{Q}}(\bm y^{k+1} ; \bm \xi^k)$
			\COMMENT{Using~\cref{alg:projection-quadric-arbitrary}}
			\STATE $\bm \xi^{k+1} \gets 2 \A \x^{k+1} +\Ab $		
			\STATE $k \gets k+1$
		\ENDWHILE
		\RETURN $\bm x^k$
	\end{algorithmic}
\end{algorithm}

This procedure is illustrated in~\cref{fig:illustration_gradient-based}.

\begin{figure}
\begin{center}
	\includegraphics[width=\textwidth]{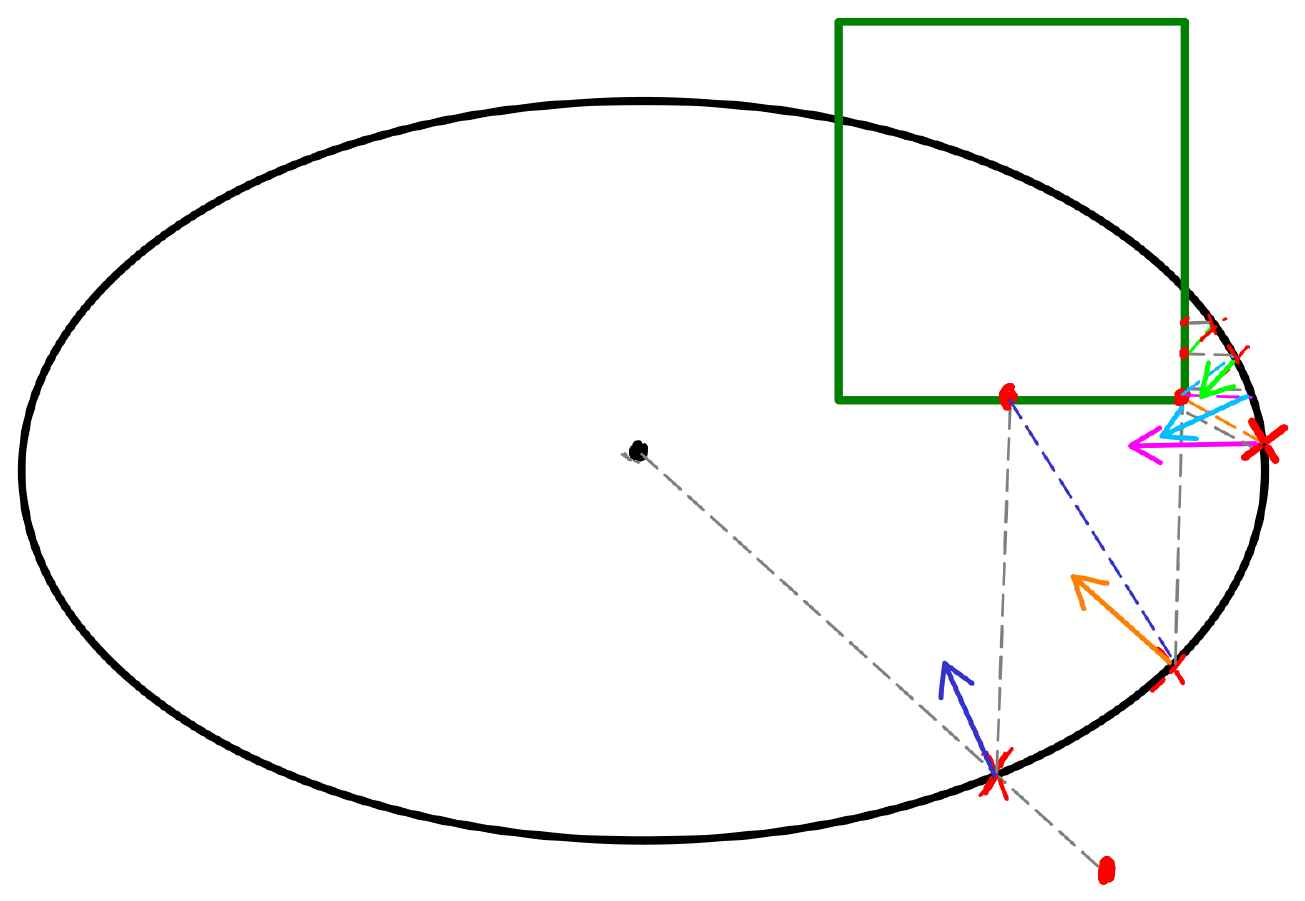}
\end{center}
\caption{Draft of the illustration of the gradient-based alternating projection.}
\label{fig:illustration_gradient-based}
\end{figure}

Note that the initial direction is the same as the APC method, and the same comment with respect to the \emph{one-shot instances} (see \S~\ref{fig:oneshot}) can be made.
